# Supplementary material for: Large scale modeling of antimicrobial resistance with interpretable classifiers
Source: arXiv:1612.01030 ancillary file (2016-12-03)
Supplement: Supplementary file 1 [file appendix.pdf]

# Large scale modeling of antimicrobial resistance with interpretable classifiers

## Appendix

Alexandre Drouin[1,3,†], Frédéric Raymond[2,3], Gaël Letarte St-Pierre[1,3], Mario Marchand[1,3], Jacques Corbeil[2,3], François Laviolette[1,3]

[1] Department of Computer Science and Software Engineering, [2] Infectious Disease Research Center, [3] Big Data Research Center
Université Laval, Québec, Canada

Table 1: Detailed description of the datasets extracted from the PATRIC database.

| **Species** | **Antibiotic** | **Genomes** | **Resistant** | **Susceptible** | **$k$-mers** |
|---|---|---|---|---|---|
| *Acinetobacter baumannii* | Amikacin | 248 | 191 | 57 | 14 111 196 |
| | Carbapenem | 232 | 122 | 110 | 35 542 666 |
| | Imipenem | 222 | 169 | 53 | 14 267 719 |
| *Mycobacterium tuberculosis* | Amikacin | 1145 | 208 | 937 | 7 589 671 |
| | Capreomycin | 1123 | 204 | 919 | 7 664 336 |
| | Cycloserine | 336 | 72 | 264 | 4 776 616 |
| | Ethambutol | 4780 | 748 | 4032 | 11 620 042 |
| | Ethionamide | 564 | 210 | 354 | 4 968 150 |
| | Isoniazid | 5022 | 1719 | 3303 | 11 688 883 |
| | Kanamycin | 1355 | 297 | 1058 | 7 604 833 |
| | Moxifloxacin | 699 | 57 | 642 | 7 176 022 |
| | Nicotinamide | 167 | 84 | 83 | 4 626 600 |
| | Ofloxacin | 851 | 307 | 544 | 5 096 831 |
| | Para-Aminosalicylic Acid | 378 | 80 | 298 | 4 873 968 |
| | Pyrazinamide | 3668 | 377 | 3291 | 10 628 165 |
| | Rifabutin | 161 | 72 | 89 | 4 672 403 |
| | Rifampin | 5022 | 1396 | 3626 | 11 670 366 |
| | Streptomycin | 3406 | 1084 | 2322 | 9 945 269 |
| *Pseudomonas aeruginosa* | Amikacin | 492 | 87 | 405 | 43 142 308 |
| | Levofloxacin | 482 | 192 | 290 | 42 783 164 |
| | Meropenem | 371 | 154 | 217 | 38 750 260 |
| *Staphylococcus aureus* | Ciprofloxacin | 1229 | 467 | 762 | 12 277 245 |
| | Clindamycin | 624 | 350 | 274 | 9 575 344 |
| | Erythromycin | 1305 | 484 | 821 | 12 408 440 |
| | Fusidic Acid | 986 | 82 | 904 | 11 929 860 |
| | Gentamicin | 1306 | 162 | 1144 | 12 409 196 |
| | Methicillin | 1593 | 707 | 886 | 13 289 281 |
| | Penicillin | 1042 | 886 | 156 | 12 051 317 |
| | Tetracycline | 1232 | 203 | 1029 | 12 279 358 |
| | Trimethoprim Sulfamethoxazole | 320 | 142 | 178 | 6 880 057 |
| *Streptococcus pneumoniae* | Beta-Lactam | 3068 | 1563 | 1505 | 17 103 512 |
| | Chloramphenicol | 409 | 149 | 260 | 6 380 123 |
| | Erythromycin | 324 | 247 | 77 | 6 252 305 |
| | Penicillin | 172 | 113 | 59 | 5 788 378 |
| | Tetracycline | 393 | 284 | 109 | 6 209 935 |
| | Trimethoprim Sulfamethoxazole | 2844 | 2203 | 641 | 16 184 170 |

[†]Corresponding author: alexandre.drouin.8@ulaval.ca

Table 2: Metrics (testing set) averaged over 10 random partitions of each dataset. These results are also illustrated in Figure 1 of the manuscript.

| Species | Antibiotic | Error rate | Sensitivity | Specificity | Rules |
|---|---|---|---|---|---|
| *Acinetobacter baumannii* | Amikacin | 0.182 | 0.873 | 0.578 | 2.000 |
| | Carbapenem | 0.078 | 0.914 | 0.929 | 2.000 |
| | Imipenem | 0.096 | 0.926 | 0.819 | 2.000 |
| | **Mean:** | **0.118** | **0.904** | **0.775** | **2.000** |
| *Mycobacterium tuberculosis* | Amikacin | 0.042 | 0.806 | 0.994 | 1.000 |
| | Capreomycin | 0.062 | 0.787 | 0.974 | 1.800 |
| | Cycloserine | 0.200 | 0.131 | 0.955 | 1.500 |
| | Ethambutol | 0.080 | 0.743 | 0.953 | 5.700 |
| | Ethionamide | 0.229 | 0.605 | 0.876 | 2.200 |
| | Isoniazid | 0.037 | 0.936 | 0.976 | 4.500 |
| | Kanamycin | 0.051 | 0.844 | 0.979 | 2.000 |
| | Moxifloxacin | 0.050 | 0.771 | 0.969 | 1.400 |
| | Nicotinamide | 0.158 | 0.746 | 0.952 | 1.000 |
| | Ofloxacin | 0.062 | 0.895 | 0.964 | 1.000 |
| | Para-Aminosalicylic Acid | 0.163 | 0.402 | 0.950 | 1.100 |
| | Pyrazinamide | 0.058 | 0.571 | 0.983 | 7.600 |
| | Rifabutin | 0.166 | 0.806 | 0.848 | 1.000 |
| | Rifampin | 0.023 | 0.963 | 0.982 | 3.500 |
| | Streptomycin | 0.095 | 0.783 | 0.961 | 6.700 |
| | **Mean:** | **0.098** | **0.719** | **0.954** | **2.800** |
| *Pseudomonas aeruginosa* | Amikacin | 0.121 | 0.506 | 0.960 | 3.200 |
| | Levofloxacin | 0.056 | 0.917 | 0.962 | 1.100 |
| | Meropenem | 0.258 | 0.647 | 0.802 | 1.100 |
| | **Mean:** | **0.145** | **0.690** | **0.908** | **1.800** |
| *Staphylococcus aureus* | Ciprofloxacin | 0.013 | 0.969 | 0.999 | 1.000 |
| | Clindamycin | 0.040 | 0.972 | 0.944 | 2.000 |
| | Erythromycin | 0.023 | 0.980 | 0.976 | 3.000 |
| | Fusidic Acid | 0.021 | 0.855 | 0.991 | 2.700 |
| | Gentamicin | 0.004 | 0.974 | 0.999 | 1.000 |
| | Methicillin | 0.012 | 0.985 | 0.990 | 1.000 |
| | Penicillin | 0.026 | 0.982 | 0.927 | 1.700 |
| | Tetracycline | 0.014 | 0.962 | 0.991 | 2.000 |
| | Trimethoprim Sulfamethoxazole | 0.036 | 0.913 | 1.000 | 1.000 |
| | **Mean:** | **0.021** | **0.955** | **0.979** | **1.711** |
| *Streptococcus pneumoniae* | Beta-Lactam | 0.215 | 0.902 | 0.663 | 9.800 |
| | Chloramphenicol | 0.049 | 0.929 | 0.962 | 1.000 |
| | Erythromycin | 0.030 | 0.970 | 0.974 | 2.100 |
| | Penicillin | 0.018 | 0.996 | 0.949 | 1.000 |
| | Tetracycline | 0.051 | 0.972 | 0.893 | 1.000 |
| | Trimethoprim Sulfamethoxazole | 0.153 | 0.972 | 0.409 | 7.500 |
| | **Mean:** | **0.086** | **0.957** | **0.808** | **3.733** |
